# Supplementary material for: Multi-Objective Intrinsic Reward Learning for Conversational Recommender Systems
Source: arXiv:2310.20109 source file (2023-10-31)
Supplement: Supplementary file 1 [file appendix.tex]

\newpage
\appendix
\section{The MDP Environment of CRS}
The MDP environment describes the current state, state transition, and the possible actions that the agent could take.

\subsection{State} The state $s_t \in \mathcal{S}$ contains all the conversation history till timestep $t$. Given a user $u$, the state is defined as,
\begin{equation}
    s_t = [\mathcal{P}^+_t, \mathcal{P}^-_t, \mathcal{V}^-_t],
\end{equation}
where (1) $\mathcal{P}^+_t$ is the set of attributes accepted by the user during the conversation; (2) $\mathcal{P}_t^-$ is the set of attributes dismissed by the user during the conversation; (3) $\mathcal{V}_t^-$ is the set of items rejected by the user. In addition, we also add the set of candidate items $\mathcal{V}^{cand}_t$  that satisfy all inquired attributes to enrich the state information. The state $s_t$ is input into a state encoder. The resulted state embedding will be concatenated with the user embedding $e_u$, which is pre-trained from given historical interaction data.

\subsection{Action} According to the state $s_t$, the agent takes an action $a_t \in \mathcal{A}$, where $a_t$ can be an item $v_t$ from the candidate item set $\mathcal{V}_t^{cand}$ to make a recommendation or an attribute $p_t$ from the candidate attribute set $\mathcal{P}_t^{cand}$ to ask attributes. Following the path reasoning approach \citep{lei2020interactive}, we identify the candidate item and candidate attribute as follows, 
\begin{align}
    \mathcal{V}_t^{cand} = \mathcal{V}_{\mathcal{P}_t^+} \setminus \mathcal{V}_t^-, \, \mathcal{P}_t^{cand} = \mathcal{P}_{\mathcal{V}_t^{cand}} \setminus 
    (\mathcal{P}_t^+ \cup \mathcal{P}_t^-),
\end{align}
where $\mathcal{V}_{\mathcal{P}_t^+}$ is the set of items satisfying all $\mathcal{P}_t^+$, and $\mathcal{P}_{\mathcal{V}_t^{cand}}$ is the set of attributes belonging to at least one of the candidate items. Specifically, when an item $v_t$ is selected by the policy, top-$K$ items with highest ranking scores will be selected to form a recommendation list $\mathcal{V}_t^{rec}$. $K$ is set to 10 in our experiments.

\subsection{State Transition} The current state $s_t$ will transit to the next state $s_{t+1}$ when the user responds to the action $a_t$. Specifically, if the agent asks an attribute $p_t$ and the user accepts it, the next state $s_{t+1}$ will be updated by $\mathcal{P}_{t+1}^+ = \mathcal{P}_t^+ \cup \{p_t\}$. Conversely, if the user rejects the attribute $p_t$, $s_{t+1}$ will be updated by $\mathcal{P}_{t+1}^- = \mathcal{P}_t^- \cup \{p_t\}$. Also, if the user rejects the recommendation $\mathcal{V}_t^{rec}$, we will update $\mathcal{V}_{t+1}^- = \mathcal{V}_t^- \cup \mathcal{V}_t^{rec}$. 

\subsection{Action Selection Strategy}
A large action search space will affect the performance of policy learning. We follow \citep{deng2021unified} to use the following two heuristics to pre-select the actions to facilitate policy learning. 
 
\textbf{Preference-based Item Selection.} We select top-$K_v$ candidate items from $\mathcal{V}_t^{cand}$ into the candidate action space $\mathcal{A}_t$ at each timestep $t$. The ranking score of an item $v$ is given by
\begin{equation}
    w_t(v) = e_u^\top e_v + \sum_{p\in \mathcal{P}_t^+}e_v^\top e_p - \sum_{p\in \mathcal{P}_t^- \cap \mathcal{P}_v} e_v^\top e_p.
        \label{eq:item_score}
\end{equation}
where $\{e_u, e_v, e_p\}$ represent the pre-trained user, item and attribute embeddings from given historical interaction data. We require $K_v \geq K$. In our experiments, both of them are set to 10.

\textbf{Weighted Entropy-based Attribute Selection.} Whereas for candidate attributes to be asked, the expected one is supposed to be
able to not only better eliminate the uncertainty of candidate items, but also encode the user preference. Inspired by \citep{lei2020interactive}, we adopt weighted entropy as the criteria to prune candidate attributes, 
\begin{align}
    w_t(p) = -\text{prob}(p_t) \cdot \log (\text{prob}(p_t)), \label{eq:weighted_entropy} \\
    \text{prob}(p_t) = \frac{\sum_{v\in \mathcal{V}_t^{cand}\cap \mathcal{V}_p} w_t(v)}{\sum_{v\in \mathcal{V}_t^{cand}} w_t(v)}, \nonumber
\end{align}
where $\mathcal{V}_p$ denotes the items that have the attribute $p$. Similar to item selection, we select top-$K_p$ candidate attributes from $\mathcal{P}_t^{cand}$ into $\mathcal{A}_t$ based on the weighted entropy score, which is set to 10 in our experiments.

\section{More Experiment Results}
A recent work \citep{hu2022learning} proposes a heuristic to identify the best action at each timestep. Specifically, they use a simple two-action policy, which only decides whether to ask an attribute question or make a recommendation. When the policy decides to ask a question, the attribute with the largest score given by Eq.\eqref{eq:weighted_entropy} will be selected. When the policy decides to recommend, the items will be ranked according to Eq.\eqref{eq:item_score} and the policy recommends the top-$K$ items. The preferred action at each timestep is decided by Algorithm \ref{alg:action_judgement} based on the authors' proposed heuristics. Then they devise the binary reward signal based on this preferred action, and use the learned reward function for policy learning. The resulted method is named as \textbf{CRIF}.

\begin{algorithm}[hpt]
\SetAlgoLined
\Require The size of candidate item set in the last turn $l_b$, the rank of target item in the last turn $k_b$, the size of candidate item set after asking an attribute $l_a$, the rank of target item after asking an attribute $k_a$, the size of candidate item set after the recommendation $l_r$, and the rank of target item after the recommendation $k_r$\;
\Ensure Action comparison result: asking an attribute is better or recommendation is better\;
Target item rank margin of ask $k_a^+=k_a - k_b$\;
Candidate item length margin of ask $l_a^+=l_a - l_b$\;
Target item rank margin of recommendation $k_r^+=k_r - k_b$\;
Candidate item length margin of recommendation $l_r^+=l_r - l_b$\;
\If {$l_b \leq 50$}{
    \If {$l_b \leq 10$}{
        \emph{recommendation better}; Exit.
    }
    \Else{
     \If{$k_a^+ > k_r^+$}{
        \emph{ask better}; Exit.
     }
     \Else{
        \emph{recommendation better}; Exit.
     }
    }
\Else{
    \If {$k_a^+ + 0.5 * l_a^+ > k_r^+ + 0.5 * l_r^+$}{
        \emph{ask better}; Exit.
    }
    \Else{
        \emph{recommendation better}. Exit.
    }
}
}

 \caption{Action Judgement of Pre-defined Rules}
 \label{alg:action_judgement}
\end{algorithm}

However, this heuristic abuses the design of user simulator that all attributes of the target item will be accepted. 
%They use this assumption to calculate the outcome of asking an attribute. But it is hardly to be reasonable in the real-world setting.  For instance, a user may favor some attributes of the target item but remain indifferent to others. 
This however creates a form of information leakage and creates an unfair advantage over the baseline solutions that do not exploit this specific knowledge. %, which explains the superior performance in the original paper. Consequently, we chose not to include it.
But it is still interesting to understand whether our learned intrinsic rewards can augment this strong heuristic. Instead of learning a reward function to match the heuristic, we directly use rules given by Algorithm \ref{alg:action_judgement} to define the extrinsic rewards: we set an action's extrinsic reward to 1 if the select action is the same as the ground-truth action given by Algorithm \ref{alg:action_judgement}; otherwise, 0. To make the problem more difficult, we set the maximum allowed turns to 10, and thus the policy needs to recommend successfully with fewer conversation turns. We first train a policy with policy gradient using the rule-based extrinsic reward, and then fine-tune the policy using \model{}.

The results are presented in Table \ref{tab:rule}. Interestingly, directly optimizing extrinsic rewards in PG+Rules already outperformed CRIF, suggesting that the estimation errors in CRIF's reward function can lead to performance degeneration. The rule-based extrinsic reward is already dense and specifically designed for conversational recommendation, yet \model{} still enhances performance generally (as seen on LastFM and Yelp*). 
However, when the pre-defined rules fit the dataset well, such as on LastFM*, the learned intrinsic rewards could be less helpful. Nevertheless, Algorithm \ref{alg:action_judgement} still contains some manually defined parts, such as the weights of $k^+$ and $l^+$, which have to be finetuned in a per-dataset basis. \model{}, by learning intrinsic rewards directly from user interactions, offers an effective augmentation to these potentially flawed handcrafted rules.

\begin{table}[tp]
\caption{Results with rule-based extrinsic reward.}
\label{tab:rule}
\resizebox{1\textwidth}{!}{
\begin{tabular}{@{}lccccccccc@{}}
\toprule
            & \multicolumn{3}{c}{LastFM} & \multicolumn{3}{c}{LastFM*}  & \multicolumn{3}{c}{Yelp*} \\ \cmidrule(l){2-10} 
            & SR@10   & AT    & hDCG    & SR@10     & AT    & hDCG      & SR@10    & AT    & hDCG   \\ \midrule
CRIF & 0.784 & 9.37 & 0.242 & 0.827 & 7.58 & 0.376   & 0.636  &  9.38 & 0.214
\\ \midrule
PG+Rules & 0.840 &  8.89 &  0.261 &   \textbf{0.952} &  \textbf{6.82} & 0.415    & 0.723 &  8.95 & 0.242
\\ \midrule 
\textbf{CRSIRL}+Rules  &   \textbf{0.862}  &   \textbf{8.84}    &   \textbf{0.274}    &  0.946 &  6.93  & \textbf{0.421}  &  \textbf{0.756} &  \textbf{8.81}  & \textbf{0.248} \\ \bottomrule
\end{tabular}
}
\end{table}

Moreover, we should note that even though \model{} is built upon the unified policy proposed in \citep{deng2021unified}, it is a general method can be easily applied to other existing RL-based CRS solutions. We additionally applied \model{} to SCPR \citep{lei2020interactive}, which reformulates the CRS problem as an interaction path reasoning process within a user-item-attribute graph. Specifically, they employ a two-action policy, which decides to ask a question or make a recommendation. The policy is optimized using the pre-defined reward described in Section 5.1. We use \model{} to fine-tune the policy obtained by SCPR. We present the results in Table \ref{tab:irl_scpr}. It shows \model{} can improve the performance significantly with the learned intrinsic rewards.

\begin{table}[h]
\vspace{-4mm}
\caption{Results of applying \model{} on SCPR.}
\label{tab:irl_scpr}
\resizebox{1\textwidth}{!}{
\begin{tabular}{@{}lccccccccc@{}}
\toprule
            & \multicolumn{3}{c}{LastFM} & \multicolumn{3}{c}{LastFM*}  & \multicolumn{3}{c}{Yelp*} \\ \cmidrule(l){2-10} 
            & SR@15    & AT    & hDCG    & SR@15     & AT    & hDCG      & SR@15    & AT    & hDCG   \\ \midrule
SCPR        &    0.465 & 12.86 & 0.139 & 0.709 & 8.43 & 0.317 & 0.489 & 12.62 & 0.159        \\ \midrule
\textbf{CRSIRL}+SCPR  &  \textbf{0.614}  &   \textbf{11.32}    &   \textbf{0.184}    & \textbf{0.773} &  \textbf{8.06} &  \textbf{0.338} &  \textbf{0.543} &  \textbf{11.02} &  \textbf{0.198}   \\ \bottomrule
\end{tabular}}
\end{table}

\bibliographystyle{plainnat}
\bibliography{reference}
